# Supplementary material for: Maximum Persistency via Iterative Relaxed Inference with Graphical Models
Source: arXiv:1508.07902 source file (2017-02-03)
Supplement: Supplementary file 2 [file experiments_suppl.tex]

\section{Detailed Experimental Evaluation}\label{sec:A-experiments}

\myparagraph{Datasets and Evaluation.} We give a brief characterization of all $38$ test problem instances and report the obtained total percentage of persistent variables of our and competing methods in Table~\ref{tab:Experiments}. 
The datasets \texttt{mrf-stereo} and \texttt{mrf-photomontage} originate from the Middlebury MRF benchmark~\cite{SzeliskiComparativeStudyMRF}. The \texttt{color-seg} and \texttt{color-seg-n4} datasets were taken from the OpenGM MRF benchmark~\cite{kappes-2015-ijcv}, \texttt{ProteinFolding} originates from~\cite{PIC2011,SideChainPredictionYanover}. All datasets are made available in the OpenGM-format~\cite{kappes-2015-ijcv}.

\par
\newcommand{\flabelw}[1]{%
    \setbox0\hbox{{\white \bf (#1)}}%
    \rlap{\hbox to \wd0{\hss\hskip1pt\bf (#1)\hss}}\box0
}
\newcommand{\flabelk}[1]{%
    \setbox0\hbox{{\bf (#1)}}%
    \rlap{\hbox to \wd0{\hss\hskip1pt\bf \white (#1)\hss}}\box0
}

\begin{figure}[t]
\centering
\setlength{\tabcolsep}{0pt}
\begin{tabular}{p{0.5\linewidth}p{0.5\linewidth}}
\begin{tabular}{c}
\begin{overpic}[tics=10,width=!,height=0.77\linewidth]{fig/exp/pfau-small-proved_sol.png}
\put (5,66){\flabelk{a}}%
\end{overpic}
\end{tabular}
&%
\begin{tabular}{c}
\begin{overpic}[tics=10,width=\linewidth,height=0.8\linewidth]{fig/exp/pfau-small-reminder-crop}
\put (5,68){\flabelk{b}}%
\end{overpic}
\end{tabular}
\end{tabular}
\caption{%
Instance {\tt pfau}. (a) Proved part of optimal solution (red solution not determined / non-unique). (b) Reminder of the optimization problem: number of remaining labels in every pixel.}
\label{fig:pfau}
\end{figure}

\begin{figure}
\centering
\setlength{\tabcolsep}{0pt}
\begin{tabular}{p{0.5\linewidth}p{0.5\linewidth}}
\begin{tabular}{c}
\begin{overpic}[tics=10,width=!,height=0.78\linewidth]{fig/exp/ted-gm-proved_sol-hatch.png}
\put (5,72){\flabelk{a}}%
\end{overpic}
\end{tabular}
&%
\begin{tabular}{c}
\begin{overpic}[tics=10,width=\linewidth,height=0.8\linewidth]{fig/exp/ted-gm-reminder-crop}
\put (5,68){\flabelk{b}}%
\end{overpic}
\end{tabular}
\end{tabular}
\caption{%
Instance {\tt ted}. (a) Proved part of optimal solution (red = solution not determined / non-unique). (b) Reminder of the optimization problem: number of remaining labels in every pixel.}
\label{fig:ted}
\end{figure}

\par
Detailed quantitative experimental evaluation can be found in Table~\ref{tab:DetailedExperimentalEvaluation}. In addition to the per-label measure of partial optimality~\eqref{measure-labels}, to allow for future comparisons we report also the {\em logarithmic measure}. It is motivated by the fact that eliminating one label in a variable with say 2 states brings more information than eliminating one label in a variable with 100 states. 
We propose to measure the total decrease of the number of configurations of the search space, \eg, from $|\X|$ to $p(|\X|)$, in the logarithmic domain:
\begin{equation}
1 - \frac{\log \prod_{v\in\V}|p_v(\X_v)|}{\log \prod_{v\in\V}|\X_v|} = 
1 - \frac{\sum_{v\in\V}\log |p_v(\X_v)|}{\sum_{v\in\V}\log|\X_v|}.
\end{equation}
\par
In Figures~\ref{fig:pfau}-\ref{fig:brain} we give examples where the method was performing well. Figures~\ref{fig:pano} and~\ref{fig:family}, on the contrary reveal some cases of very poor performance. For example for {\tt photomontage/pano} instance, we report $80\%$ solution completeness, but these $80\%$ only correspond to trivial hard constraints in the problem. Other methods perform worse mainly because they consider determining complete optimal labels only (\PBPTRWS) or intervals of labels (\MQPBO).

\begin{figure}
\centering
\setlength{\tabcolsep}{0pt}
\begin{overpic}[tics=10,width=\linewidth]{fig/exp/brain-0-proved_sol.png}
\end{overpic}
\caption{
Instance {\tt brain-9mm/brain-0}. Slices of the 3D volumetric problem. Proved part of optimal solution (red = solution not determined / non-unique).
}
\label{fig:brain}
\end{figure}

\begin{figure}[!t]
\centering
\setlength{\tabcolsep}{0pt}
\begin{tabular}{p{0.5\linewidth}p{0.5\linewidth}}
\begin{overpic}[tics=10,width=\linewidth,height=0.8\linewidth]{fig/exp/pano-gm-labeling.png}
\put (5,68){\flabelw{a}}%
\end{overpic}
&%
\begin{overpic}[tics=10,width=\linewidth,height=0.8\linewidth]{fig/exp/pano-gm-labeling1-rc.png}
\put (5,68){\flabelw{b}}%
\end{overpic}\\
\begin{tabular}{c}
\begin{overpic}[tics=10,width=\linewidth,height=0.77\linewidth]{fig/exp/pano-gm-proved_sol.png}
\put (5,68){\flabelw{c}}%
\end{overpic}
\end{tabular}
&%
\begin{tabular}{c}
\begin{overpic}[tics=10,width=\linewidth,height=0.8\linewidth]{fig/exp/pano-gm-reminder-crop}
\put (5,68){\flabelw{d}}%
\end{overpic}
\end{tabular}
\end{tabular}
\caption{
Instance {\tt pano}: label encodes the image index for photomontage. (a) (b) Two labelings by TRW-S with slightly different initializations. It is clear that there is high ambiguity.
(c) Part of the solution that was proved optimal and unique. 
(d) Reminder of the optimization problem (number of non-eliminated labels).
It is clear that the method essentially removed hard constraints implied by different fields of view of images composing the panorama.
}
\label{fig:pano}
\end{figure}

\begin{figure}[!t]
\centering
\setlength{\tabcolsep}{0pt}
\begin{tabular}{p{0.5\linewidth}p{0.5\linewidth}}
\begin{overpic}[tics=10,width=\linewidth,height=0.8\linewidth]{fig/exp/family-gm-labeling.png}
\put (5,68){(a)}%
\end{overpic}
&%
\begin{overpic}[tics=10,width=\linewidth,height=0.8\linewidth]{fig/exp/family-gm-reminder-crop}
\put (5,68){(b)}%
\end{overpic}
\end{tabular}
\caption{
Instance {\tt family}. (a) Labeling by TRW-S. (b) Reminder of the optimization problem (number of labels per pixel). It is clear that the method essentially only followed the hard constraints corresponding to the scribbles provided by the user and constrained very few pixels ontop of that.
}
\label{fig:family}
\end{figure}
